# Supplementary material for: Multimodal Large Language Models for Phishing Webpage Detection and Identification
Source: arXiv:2408.05941 source file (2024-08-12)
Supplement: Supplementary file 1 [file appendix.tex]

\appendix
\addcontentsline{toc}{section}{Appendices}

\section*{Appendix}

\begin{mdframed}
\texttt{Brand: Alibaba,}\\
\texttt{Has Credentials'': Yes,}\\
\texttt{Has Call To Actions: Yes,}\\
\texttt{List of Credentials fields: Email address or member ID, Password,}\\
\texttt{List of Call-To-Actions: Sign In button, Create account link, Forgot password? link,}\\
\texttt{Confidence Score: 10.00,}\\
\texttt{Supporting Evidence: The identification of the brand ``Alibaba'' is} \texttt{confidently based on multiple indicators from the provided screenshot and HTML information. The screenshot prominently displays the Alibaba.com logo alongside distinctive branding elements like color scheme and promotional content. Further corroboration comes from the HTML data, which includes a title (``Alibaba Manufacturer Directory - Suppliers, Manufacturers, Exporters \& Importers''), and footer text which repeatedly references Alibaba.com and associated Alibaba Group entities like Taobao, Tmall.com, and Alipay. Additionally, the inclusion of a favicon URL containing `alicdn.com', which is known to be associated with Alibaba, solidifies the brand identification. The presence of fields for credentials (email or member ID and password) and multiple call-to-action elements (such as the sign-in and create account options) are clear from both the screenshot and HTML headers and span texts.''}
\end{mdframed}

\vspace{0.4cm}
\textit{\textbf{Supporting Evidence:}}
\vspace{0.2cm}
\begin{mdframed}
The brand \"wBay\" is prominently displayed at the top of the webpage, reinforcing it as the primary identity. The screenshot indicates the functionality for user login with fields specifically labeled for \"User IC\" and \"Password,\" which suggests that sensitive user credentials are being requested. There are clear call-to-action buttons for \"Sign in\" and \"Register,\" directing user interaction explicitly. The presence of another similar brand referenced in a promotional graphic (\"Go on a selling spree with eBay\") within the same page could potentially confuse the direct brand identity. However, the overarching and repeated reference to \"wBay\" in formal text areas such as the page title and footer copyright clarifies the brand being \"wBay.\" This evidence strongly points to \"wBay\" as the intended brand representation on this webpage.
\textbf{\textit{<Response format instruction as same as the prompt for screenshot>}}
\end{mdframed}

\subsection{Prompting}
\todo{Prompt template of each LLM, if there is any difference}

% \begin{table}[t]
%     \caption{System Prompt for HTML}
%     \centering
%     \begin{tabular}{ c }
%     \toprule
%     System Prompt - HTML     
%     \midrule
%     I want you to act as a webpage brand identifier. \\
%     Given the key information from the html script of a webpage. I want you to identify the brand of the webpage from this info alone.  The key information is extracted from the actual html script of the webpage, and this information includes the title of the webpage, the metadata, the favicon, the logo attribute, the footer, and header text, as well as the nav bar. These areas are where the brand information can normally be found. Make good use of this information to identify the brand related to each.    
%     \bottomrule
%     \end{tabular}
%     \label{tab:system_prompt_default}
%     \vspace{-0.3cm}
% \end{table}

\textbf{System Prompt - HTML} \\
I want you to act as a webpage brand identifier.
Given the key information from the HTML script of a webpage, I want you to identify the brand of the webpage from this information alone. The key information is extracted from the actual HTML script of the webpage, and this information includes the title of the webpage, the metadata, the favicon, the logo attribute, the footer and header text, and the nav bar. These areas are where the brand information can typically be found. Make good use of this information to identify the brand related to each.\\

\textbf{System Prompt - Screenshot}\\
I want you to act as a webpage brand identifier.\\
Given a screenshot of a webpage. I want you to identify the brand of the webpage from the screenshot alone. \\
Additionally, also note whether fields are asking for sensitive user credentials as well as any call-to-action buttons/links.\\
Examples of sensitive user credentials: email, username, password, phone number, etc.\\
Examples of call-to-action elements: buttons or links that lead to asking for user credentials. \\

\textbf{System Prompt - Screenshot and HTML} \\
I want you to act as a webpage brand identifier.
Given a screenshot and key information from the HTML script of a webpage. I want you to identify the brand of the webpage from these two sources alone. 
Additionally, also note whether there are fields asking for sensitive user credentials as well as any call-to-action buttons/links.
Examples of sensitive user credentials: email, username, password, phone number, etc.
Examples of call-to-action elements: buttons or links that lead to asking for user credentials. 
\\\\

\textbf{Shared Part among all configurations}\\
Please adhere strictly to the following rules for your analysis:\\
1. Do not interact with the webpage in a live environment or use browser functionalities.\\
2. Avoid inspecting the webpage's source code, the website's address bar, SSL certificates, URLs, or any interactive features.\\
3. Your analysis should be grounded solely on the information from the html script. \\
4. No additional resources or external validations should be used. \\

Take note that some pages may include information/logos of other brands, especially pages that use single sign-on features or pages created by website builder. \\ \\

\textbf{Response Format} \\
    Return your response in the following format, and replace everything in < > with your answer:\\
    1. Brand: <response>\\
    2. Has\_Credentials: <Yes/No>\\
    3. Has\_Call\_To\_Action: <Yes/No>\\
    4. List\_of\_credentials: <response if Yes for (2), otherwise NA. Keep within the top 10 fields.>\\
    5. List\_of\_call\_to\_action: <response if Yes for (3), otherwise NA. Keep within the top 10 fields.>\\
    6. Confidence\_Score: <How confident are you when identifying the brand on a scale of 0.00 to 10.00 (give in 2 decimal places), 10.00 being absolutely confident, 0.00 being not confident>\\
    7. Supporting\_Evidence: <response, keep it within 300 words>\\

\textbf{Response Format - HTML} \\1
Return your response in the following format, replace everything in <> with your answer:\\
1. Brand: <response> \\
2. Confidence\_Score: <How confident are you when identifying the brand on scale of 0.00 to 10.00 (in 2 decimal places), 10.00 being absolutely confident, 0.00 being not confident> \\
3. Supporting\_Evidence: <response, keep it within 300 words> \\

\textbf{Chain of Thought}\\
Analyze the webpage screenshot by following these steps:\\
1. Identify the webpage brand based on information available from the html script. \\
2. The brand can be obtained from any part of the information (i.e., title, meta\_description, favicon, logo, footer, header, nav\_bar\_content, paragraph, text)\\
3. Most of the time you will be able to identify it from the title or footer information. \\
4. If you cannot find or identify the brand, return NA for 'brand' in your response.\\
5. Provide a comprehensive evaluation of the html script. Include a detailed explanation for your analysis.\\
6. Take note of how confident you are in identifying the brand.\\

\textbf{Chain of Thought - HTML}\\
Analyze the webpage screenshot by following these steps:\\
1. Identify the webpage brand based on information available from the html script. \\
2. The brand can be obtained from any part of the information (i.e., title, meta\_description, favicon, logo, footer, header, nav\_bar\_content, paragraph, text)\\
3. Most of the time you will be able to identify it from the title or footer information. \\
4. If you cannot find or identify the brand, return NA for 'brand' in your response.\\
5. Provide a comprehensive evaluation of the html script. Include a detailed explanation for your analysis.\\
6. Take note of how confident you are in identifying the brand.\\
